# Supplementary material for: Identifying Hosts of Families of Viruses: A Machine Learning Approach
Source: arXiv:1105.5821 ancillary file (2011-05-29)
Supplement: Supplementary file 1 [file list_of_viruses.pdf]

Table 1: List of viruses in *Rhabdoviridae* family used in learning.

| Identifier | Name                                               | Host   | Subfamily         |
|------------|----------------------------------------------------|--------|-------------------|
| NC_009609  | Orchid fleck virus RNA 2                           | Plant  | unassigned        |
| NC_006942  | Taro vein chlorosis virus                          | Plant  | Nucleorhabdovirus |
| NC_005975  | Maize mosaic virus                                 | Plant  | Nucleorhabdovirus |
| EF614258   | West Caucasian bat virus                           | Animal | Lyssavirus        |
| DQ186554   | Iranian maize mosaic nucleorhabdovirus             | Plant  | Nucleorhabdovirus |
| NC_007642  | Lettuce necrotic yellows virus                     | Plant  | Cytorhabdovirus   |
| EF687738   | Lettuce yellow mottle virus                        | Plant  | Cytorhabdovirus   |
| NC_002251  | Northern cereal mosaic virus                       | Plant  | Cytorhabdovirus   |
| NC_001615  | Sonchus yellow net virus                           | Plant  | Cytorhabdovirus   |
| NC_005974  | Maize fine streak virus                            | Plant  | Nucleorhabdovirus |
| NC_003746  | Rice yellow stunt virus                            | Plant  | Nucleorhabdovirus |
| DQ491000   | Spring viremia of carp virus isolate A2            | Animal | Vesiculovirus     |
| EU373657   | Cocal virus Indiana 2                              | Animal | Vesiculovirus     |
| AJ318079   | Spring Viremia of Carp                             | Animal | Vesiculovirus     |
| NC_002803  | Spring viremia of carp virus                       | Animal | Vesiculovirus     |
| AF104985   | Hirame rhabdovirus strain CA 9703                  | Animal | Novirhabdovirus   |
| NC_005093  | Hirame rhabdovirus                                 | Animal | Novirhabdovirus   |
| EU177782   | Spring viremia of carp virus isolate BJ0505-2      | Animal | Vesiculovirus     |
| EU373658   | Vesicular stomatitis Alagoas virus Indiana 3       | Animal | Vesiculovirus     |
| AJ810084   | Isfahan virus N gene                               | Animal | Vesiculovirus     |
| DQ097384   | Spring viremia of carp virus isolate A1            | Animal | Vesiculovirus     |
| NC_001652  | Infectious hematopoietic necrosis virus            | Animal | Novirhabdovirus   |
| X89213     | Infectious haematopoietic necrosis virus (IHNV)    | Animal | Novirhabdovirus   |
| NC_000855  | Viral hemorrhagic septicemia virus                 | Animal | Novirhabdovirus   |
| Y18263     | Viral hemorrhagic septicemia virus strain Fil3 RNA | Animal | Novirhabdovirus   |
| AY840978   | Tupaia rhabdovirus                                 | Animal | Dimarhabdovirus   |
| NC_007020  | Tupaia rhabdovirus                                 | Animal | Dimarhabdovirus   |
| NC_008514  | Siniperca chuatsi rhabdovirus                      | Animal | Dimarhabdovirus   |
| DQ399789   | Siniperca chuatsi rhabdovirus from China           | Animal | Dimarhabdovirus   |
| AF147498   | Snakehead rhabdovirus                              | Animal | Novirhabdovirus   |
| NC_000903  | Snakehead rhabdovirus                              | Animal | Novirhabdovirus   |
| AF081020   | Australian bat lyssavirus                          | Animal | Lyssavirus        |
| EF614261   | Khujiand lyssavirus                                | Animal | Lyssavirus        |
| EF614259   | Aravan virus                                       | Animal | Lyssavirus        |
| AF418014   | Australian bat lyssavirus                          | Animal | Lyssavirus        |
| EU293116   | Rabies virus isolate 9704ARG                       | Animal | Lyssavirus        |
| EU293115   | Rabies virus isolate 9147FRA                       | Animal | Lyssavirus        |
| EU293121   | Rabies virus isolate 8743THA                       | Animal | Lyssavirus        |
| EU293114   | European bat lyssavirus 2 isolate 9018HOL          | Animal | Lyssavirus        |
| NC_009528  | European bat lyssavirus 2                          | Animal | Lyssavirus        |
| NC_001542  | Rabies virus                                       | Animal | Lyssavirus        |
| NC_006429  | Mokola virus                                       | Animal | Lyssavirus        |
| EU293117   | Mokola virus isolate 86100CAM                      | Animal | Lyssavirus        |
| EU293118   | Mokola virus isolate 86101RCA                      | Animal | Lyssavirus        |
| NC_009527  | European bat lyssavirus 1                          | Animal | Lyssavirus        |
| EF614260   | Irkut virus                                        | Animal | Lyssavirus        |
| EU293110   | Lagos bat virus isolate 8619NGA                    | Animal | Lyssavirus        |
| EU293108   | Lagos bat virus isolate 0406SEN                    | Animal | Lyssavirus        |
| NC_002526  | Bovine ephemeral fever virus                       | Animal | Ephemerovirus     |

Table 2: List of viruses in *Picornaviridae* family used in learning.

| Identifier | Name                                                | Host         | Subfamily   |
|------------|-----------------------------------------------------|--------------|-------------|
| NC_014137  | Honey bee slow paralysis virus                      | Invertebrate | Cripavirus  |
| NC_001366  | Theilovirus                                         | Vertebrate   | Cardiovirus |
| NC_003005  | Taura syndrome virus                                | Invertebrate | Cripavirus  |
| NC_003783  | Triatoma virus                                      | Invertebrate | Cripavirus  |
| NC_003077  | Equine rhinitis B virus 2                           | Vertebrate   | Erbovirus   |
| NC_001834  | Drosophila C virus                                  | Invertebrate | Cripavirus  |
| NC_003784  | Black queen cell virus                              | Invertebrate | Cripavirus  |
| NC_002066  | Sacbrood virus                                      | Invertebrate | Iflavirus   |
| NC_008182  | Black raspberry necrosis virus RNA1                 | Plant        | Cripavirus  |
| NC_013115  | Human enterovirus 107                               | Vertebrate   | Enterovirus |
| NC_013114  | Human enterovirus 98                                | Vertebrate   | Enterovirus |
| NC_005092  | Ectropis obliqua picorna-like virus                 | Invertebrate | unassigned  |
| NC_013695  | Simian picornavirus strain N203                     | Vertebrate   | Enterovirus |
| NC_010384  | Simian picornavirus strain N125                     | Vertebrate   | Enterovirus |
| NC_008183  | Black raspberry necrosis virus RNA2                 | Plant        | Cripavirus  |
| NC_011829  | Porcine kobuvirus swine/S-1-HUN/2007/Hungary        | Vertebrate   | Kobuvirus   |
| NC_013755  | Kobuvirus pig/JY-2010a/CHN                          | Vertebrate   | Kobuvirus   |
| NC_012986  | Human klassevirus 1                                 | Vertebrate   | unassigned  |
| NC_012957  | Salivirus NG-J1                                     | Vertebrate   | unassigned  |
| NC_011190  | Mikania micrantha mosaic virus RNA1                 | Plant        | Cripavirus  |
| NC_011189  | Mikania micrantha mosaic virus RNA2                 | Plant        | Cripavirus  |
| NC_010354  | Bovine rhinitis B virus                             | Vertebrate   | Erbovirus   |
| NC_008250  | Duck hepatitis A virus                              | Vertebrate   | Hepatovirus |
| NC_006553  | Avian sapelovirus                                   | Vertebrate   | Sapelovirus |
| NC_013219  | Turnip ringspot virus RNA 2                         | Plant        | Cripavirus  |
| NC_013218  | Turnip ringspot virus RNA 1                         | Plant        | Cripavirus  |
| NC_011451  | Foot-and-mouth disease virus - type SAT 1           | Vertebrate   | Aphthovirus |
| NC_011450  | Foot-and-mouth disease virus - type A               | Vertebrate   | Aphthovirus |
| NC_005266  | Raspberry ringspot virus RNA1                       | Plant        | Cripavirus  |
| NC_003992  | Foot-and-mouth disease virus - type SAT 2           | Vertebrate   | Aphthovirus |
| NC_004915  | Foot-and-mouth disease virus - type Asia 1          | Vertebrate   | Aphthovirus |
| NC_004807  | Kashmir bee virus                                   | Invertebrate | Cripavirus  |
| NC_004451  | Simian picornavirus 1                               | Vertebrate   | unassigned  |
| NC_004365  | Aphid lethal paralysis virus                        | Invertebrate | Cripavirus  |
| NC_004004  | Foot-and-mouth disease virus - type O               | Vertebrate   | Aphthovirus |
| NC_003987  | Porcine enterovirus 8                               | Vertebrate   | Enterovirus |
| NC_003924  | Cricket paralysis virus                             | Invertebrate | Cripavirus  |
| NC_003113  | Perina nuda virus                                   | Invertebrate | Iflavirus   |
| NC_002554  | Foot-and-mouth disease virus - type C               | Vertebrate   | Aphthovirus |
| NC_001874  | Rhopalosiphum padi virus                            | Invertebrate | Cripavirus  |
| NC_001490  | Human rhinovirus 14                                 | Vertebrate   | Rhinovirus  |
| NC_001479  | Encephalomyocarditis virus                          | Vertebrate   | Cardiovirus |
| NC_012212  | Chaetoceros socialis f. radians RNA virus segment 1 | Plant        | Cripavirus  |
| NC_012802  | Human cosavirus D1                                  | Vertebrate   | unassigned  |
| NC_012801  | Human cosavirus B1                                  | Vertebrate   | unassigned  |
| NC_012800  | Human cosavirus A1                                  | Vertebrate   | unassigned  |
| NC_012798  | Human cosavirus E1                                  | Vertebrate   | unassigned  |
| NC_010411  | Simian picornavirus 17                              | Vertebrate   | unassigned  |
| NC_003446  | Strawberry mottle virus RNA 2                       | Plant        | Cripavirus  |
| NC_003445  | Strawberry mottle virus RNA 1                       | Plant        | Cripavirus  |
| NC_010415  | Simian enterovirus SV6                              | Vertebrate   | Enterovirus |

|           |                                          |              |             |
|-----------|------------------------------------------|--------------|-------------|
| NC_010413 | Simian enterovirus SV43                  | Vertebrate   | Enterovirus |
| NC_010412 | Simian enterovirus SV19                  | Vertebrate   | Enterovirus |
| NC_003792 | Cycas necrotic stunt virus RNA 2         | Plant        | Cripavirus  |
| NC_003791 | Cycas necrotic stunt virus RNA 1         | Plant        | Cripavirus  |
| NC_010988 | Tomato marchitez virus RNA 2             | Plant        | Cripavirus  |
| NC_010987 | Tomato marchitez virus RNA 1             | Plant        | Cripavirus  |
| NC_009891 | Seal picornavirus type 1                 | Vertebrate   | unassigned  |
| NC_009758 | Marine RNA virus JP-B                    | Plant        | unassigned  |
| NC_009757 | Marine RNA virus JP-A                    | Plant        | unassigned  |
| NC_009530 | Brevicoryne brassicae picorna-like virus | Invertebrate | unassigned  |
| NC_009448 | Saffold virus                            | Vertebrate   | Cardiovirus |
| NC_009032 | Tomato torrado virus RNA2                | Plant        | Cripavirus  |
| NC_009013 | Tomato torrado virus RNA1                | Plant        | Cripavirus  |
| NC_006964 | Strawberry latent ringspot virus RNA1    | Plant        | Cripavirus  |
| NC_005281 | Heterosigma akashiwo RNA virus SOG263    | Plant        | Marnavirus  |
| NC_005097 | Tobacco ringspot virus RNA 1             | Plant        | Cripavirus  |
| NC_005096 | Tobacco ringspot virus RNA 2             | Plant        | Cripavirus  |
| NC_004439 | Tomato black ring virus RNA 1            | Plant        | Cripavirus  |
| NC_004421 | Bovine kobuvirus                         | Vertebrate   | Kobuvirus   |
| NC_003988 | Simian enterovirus A                     | Vertebrate   | Enterovirus |
| NC_003983 | Equine rhinitis B virus 1                | Vertebrate   | Erbovirus   |
| NC_003974 | Patchouli mild mosaic virus RNA 2        | Plant        | Cripavirus  |
| NC_003840 | Tomato ringspot virus RNA 1              | Plant        | Cripavirus  |
| NC_003839 | Tomato ringspot virus RNA 2              | Plant        | Cripavirus  |
| NC_003788 | Apple latent spherical virus segment 2   | Plant        | Cripavirus  |
| NC_003787 | Apple latent spherical virus segment 1   | Plant        | Cripavirus  |
| NC_003741 | Red clover mottle virus RNA 1            | Plant        | Cripavirus  |
| NC_003738 | Red clover mottle virus RNA 2            | Plant        | Cripavirus  |
| NC_003694 | Beet ringspot virus RNA 2                | Plant        | Cripavirus  |
| NC_003693 | Beet ringspot virus RNA 1                | Plant        | Cripavirus  |
| NC_003622 | Grapevine chrome mosaic virus RNA 1      | Plant        | Cripavirus  |
| NC_003621 | Grapevine chrome mosaic virus RNA 2      | Plant        | Cripavirus  |
| NC_003615 | Grapevine fanleaf virus RNA 1            | Plant        | Cripavirus  |
| NC_003550 | Cowpea mosaic virus RNA 2                | Plant        | Cripavirus  |
| NC_003549 | Cowpea mosaic virus RNA 1                | Plant        | Cripavirus  |
| NC_003509 | Blackcurrant reversion virus RNA1        | Plant        | Cripavirus  |
| NC_003502 | Blackcurrant reversion virus RNA 2       | Plant        | Cripavirus  |
| NC_003545 | Cowpea severe mosaic virus RNA 1         | Plant        | Cripavirus  |
| NC_003544 | Cowpea severe mosaic virus RNA 2         | Plant        | Cripavirus  |
| NC_003975 | Patchouli mild mosaic virus RNA 1        | Plant        | Cripavirus  |
| NC_010710 | Radish mosaic virus RNA2                 | Plant        | Cripavirus  |
| NC_010709 | Radish mosaic virus RNA1                 | Plant        | Cripavirus  |
| NC_009996 | Human rhinovirus C                       | Vertebrate   | Rhinovirus  |
| NC_009887 | Human enterovirus 100                    | Vertebrate   | Enterovirus |
| NC_009750 | Duck hepatitis virus AP                  | Vertebrate   | Hepatovirus |
| NC_009025 | Israel acute paralysis virus of bees     | Invertebrate | Cripavirus  |
| NC_006965 | Strawberry latent ringspot virus RNA2    | Plant        | Cripavirus  |
| NC_006272 | Cherry rasp leaf virus RNA2              | Plant        | Cripavirus  |
| NC_006271 | Cherry rasp leaf virus                   | Plant        | Cripavirus  |
| NC_006057 | Arabis mosaic virus RNA 1                | Plant        | Cripavirus  |
| NC_006056 | Arabis mosaic virus RNA 2                | Plant        | Cripavirus  |
| NC_005290 | Broad bean wilt virus 1 RNA 2            | Plant        | Cripavirus  |
| NC_005289 | Broad bean wilt virus 1 RNA 1            | Plant        | Cripavirus  |
| NC_005267 | Raspberry ringspot virus RNA 2           | Plant        | Cripavirus  |

|           |                                          |              |              |
|-----------|------------------------------------------|--------------|--------------|
| NC_004830 | Deformed wing virus                      | Invertebrate | Cripavirus   |
| NC_004441 | Porcine enterovirus B                    | Vertebrate   | Enterovirus  |
| NC_004440 | Tomato black ring virus RNA 2            | Plant        | Cripavirus   |
| NC_003990 | Avian encephalomyelitis virus            | Vertebrate   | Tremovirus   |
| NC_003985 | Porcine teschovirus 1                    | Vertebrate   | Teschovirus  |
| NC_003982 | Equine rhinitis A virus                  | Vertebrate   | Aphthovirus  |
| NC_003976 | Ljungan virus                            | Vertebrate   | Parechovirus |
| NC_003800 | Squash mosaic virus RNA 2                | Plant        | Cripavirus   |
| NC_003799 | Squash mosaic virus RNA 1                | Plant        | Cripavirus   |
| NC_003782 | Himetobi P virus                         | Invertebrate | Cripavirus   |
| NC_003781 | Infectious flacherie virus               | Invertebrate | Iflavirus    |
| NC_003628 | Parsnip yellow fleck virus               | Plant        | Sequivirus   |
| NC_003626 | Maize chlorotic dwarf virus              | Plant        | Waikivirus   |
| NC_003623 | Grapevine fanleaf virus RNA 2            | Plant        | Cripavirus   |
| NC_003496 | Bean pod mottle virus RNA 1              | Plant        | Cripavirus   |
| NC_003495 | Bean pod mottle virus RNA 2              | Plant        | Cripavirus   |
| NC_003004 | Broad bean wilt virus 2 RNA2             | Plant        | Cripavirus   |
| NC_003003 | Broad bean wilt virus 2 RNA1             | Plant        | Cripavirus   |
| NC_002548 | Acute bee paralysis virus                | Invertebrate | Cripavirus   |
| NC_001918 | Aichi virus                              | Vertebrate   | Kobuvirus    |
| NC_001897 | Human parechovirus                       | Vertebrate   | Parechovirus |
| NC_001859 | Bovine enterovirus                       | Vertebrate   | Enterovirus  |
| NC_001632 | Rice tungro spherical virus              | Plant        | Waikavirus   |
| NC_001617 | Human rhinovirus 89                      | Vertebrate   | Rhinovirus   |
| NC_001612 | Human enterovirus A                      | Vertebrate   | Enterovirus  |
| NC_002058 | Poliovirus                               | Vertebrate   | Enterovirus  |
| NC_001489 | Hepatitis A virus                        | Vertebrate   | Parechovirus |
| NC_001472 | Human enterovirus B                      | Vertebrate   | Enterovirus  |
| NC_001430 | Human enterovirus D                      | Vertebrate   | Enterovirus  |
| NC_001428 | Human enterovirus C                      | Vertebrate   | Enterovirus  |
| NC_005876 | Kakugo virus                             | Invertebrate | Iflavirus    |
| NC_003779 | Plautia stali intestine virus            | Invertebrate | Cripavirus   |
| NC_010810 | Human TMEV-like cardiovirus              | Vertebrate   | Cardiovirus  |
| NC_011349 | Seneca valley virus                      | Vertebrate   | Senecavirus  |
| NC_007522 | Schizochytrium single-stranded RNA virus | Plant        | unassigned   |
| NC_006559 | Solenopsis invicta virus 1               | Invertebrate | Cripavirus   |
| NC_003785 | Satsuma dwarf virus RNA 1                | Plant        | Cripavirus   |
| NC_003786 | Satsuma dwarf virus RNA 2                | Plant        | Cripavirus   |
| NC_008029 | Homalodisca coagulata virus-1            | Invertebrate | Cripavirus   |
